# Supplementary material for: A Central Limit Theorem for Algorithmic Estimator of Saddle Point
Source: arXiv:2306.06305 source file (2023-11-05)
Supplement: Supplementary file 3 [file old_appendix.tex]

                             %% This removes title for more space 
          %% Your response goes here (at most one page pdf).
          We thank all the reviewers. Due to lack of space, our answers are brief. Please reach out to us for further clarification. 
          \textcolor{Purple0}{A=Assumption}\textbf{ MC=Markov Chain,SC=Strongly-convex,PJ92=Polyak-Juditsky 1992.}
           \textbf{\color{red}{Novelty} } For the state-dependent Markov noise, showing the stability of the dynamics, which is essential for a.s. convergence (Thm 7,11), is non-trivial (explained after Lemma 6). It requires to modify SEG and establish that tail probability of the number of reinitializations $T_k$ decrease exponentially through a carefully constructed event $\mathcal{A}$ (not needed in PJ92). Unlike PJ92, proof of CLT (Thm 12) depends on constructing an auxiliary chain $\tilde{z}_k$ and a different noise decomposition. We use $\|z_k-z^*\|_2^2$ as Lyapounov function instead of $f(z_k)-f(z^*)$ in stochastic minimization as it is meaningless in SPP. For the martingale-difference noise the proof techniques are similar to PJ92 as stated in our proof although the CLT has not been explicitly proved before. \textbf{\color{red}{On A5.1}} 
          \textcolor{Purple0}{A5.1.1} is the drift condition and \textcolor{Purple0}{A5.1.2-5.1.3} are regularity conditions on the MC. \textcolor{Purple0}{A5.1.1} is required for the chain to be V-uniformly ergodic for fixed $z$.
          \textbf{In Application:} The state-dependent Markov noise, and \textcolor{Purple0}{A5.1} arises in numerous applications (ref. in Sec 2): strategic classification with adaptive best response (\textcolor{Purple0}{A2,4,5} in Li and Wai, 2022, verified in Example 1); policy gradient (\textcolor{Purple0}{A5,A6,A7} in Karimi et al., 2019), and actor-critic algorithm in reinforcement learning (\textcolor{Purple0}{A4.2} and \textcolor{Purple0}{4.3} in [3] below); MLE with missing data (Example 4, Liang, 2010); multitask strategic classification, and relative cost maximization in competitive markets (\textcolor{Purple0}{A2,3,5} in Wood and Dall’Anese, 2022, \textcolor{Purple0}{A5} implies our \textcolor{Purple0}{A5.1.1} as shown in [4] below). A few of the above works assume uniform ergodicity whereas we assume weaker $\mathcal{V}$-uniform ergodicity.
          \textbf{In Theory:} 
          \textcolor{Purple0}{A5.1.1} is widely used in MC theory (e.g. see Ch. 15 of the book Meyn \& Tweedie 2012[2], 14.1 in Douc et al., 2018 [5] apart from the references cited in our work).
          \textbf{\textcolor{blue}{R\#7}}
1. The work is extendable to SGDA and we conjecture similar results will hold. This work is intended to pave the way for CLT for convex-concave problems where SGDA can diverge unlike SEG. 
2. State-dependent MC is defined in the first line of \textcolor{Purple0}{A5.1}. We will take it out in the final version. Since $z_k\to z^*$ a.s., the stationary distribution of the MC corresponds to $z^*$. 
\textbf{\textcolor{blue}{R\#9}}
          \textbf{Correctness: The proof is correct.} It follows from Kronecker's Lemma as mentioned just after (37). Details: 
          From Lemma 14 we have, 
          $\|\sum_{i=j}^kY_j^i\|_2\lesssim j^a$.
          Then, using the eqn two lines above (36), and that we choose $\eta_j=j^{-a}$, we have 
          $\|T_4\|_2\leq k^{-1/2}\sum_{j=1}^k\eta_j\|\sum_{i=j}^kY_j^i\|_2\|H(z_{j-1})-Q^*V_{j-1}\|_2\lesssim k^{-1/2}\sum_{j=1}^k\|H(z_{j-1})-Q^*V_{j-1}\|_2$. Now, using Assumption 3.4, and that $z_k\to z^*$ almost surely, for sufficiently large $k$ we have,
          $\|T_4\|_2\lesssim k^{-1/2}\sum_{j=1}^k\|z_{j-1}-z^*\|_2^2$. Now we will use Kronecker's Lemma to show $k^{-1/2}\sum_{j=1}^k\|z_{j-1}-z^*\|_2^2\to 0$. First we state Kronecker's Lemma.
          \textbf{Kronecker's Lemma} \textit{Let $\{x_j\}$ be a real sequence such that $\sum_{j=1}^\infty x_j<\infty$, then, for any non-decreasing positive sequence $\{b_j\}$ such that $b_j\to\infty$ one has, $\lim_{k\to\infty}b_k^{-1}\sum_{j=1}^{k}b_jx_j=0$.} 
          Now, set $b_j=\sqrt{j}$, $x_j=j^{-1/2}\|z_{j-1}-z^*\|_2^2$. In (37) in the paper, we have shown, $\sum_{j=1}^{\infty}j^{-1/2}\|z_{j-1}-z^*\|_2^2<\infty$. Then, using Kronecker's Lemma, we get, $k^{-1/2}\sum_{j=1}^k\|z_{j-1}-z^*\|_2^2\to 0$.
          \textcolor{Purple0}{A3.4} and Lm. 14, $\|T_4\|_2\leq k^{-1/2}\sum_{j=1}^k\eta_j\|\sum_{i=j}^kY_j^i\|_2\|H(z_{j-1})-Q^*V_{j-1}\|_2\lesssim k^{-1/2}\sum_{j=1}^k\eta_jj^a\|z_{j-1}-z^*\|_2^2\lesssim k^{-1/2}\sum_{j=1}^k\|z_{j-1}-z^*\|_2^2$. Now we state \textbf{Kronecker Lemma} \textit{Let $\{x_j\}$ be a real sequence such that $\sum_{j=1}^\infty x_j<\infty$, then, for any non-decreasing positive sequence $\{b_j\}$ such that $b_j\to\infty$ one has, $\lim_{k\to\infty}b_k^{-1}\sum_{j=1}^{k}b_jx_j=0$.} Setting $b_j=\sqrt{j}$, $x_j=j^{-1/2}\|z_{j-1}-z^*\|_2^2$ we get, $k^{-1/2}\sum_{j=1}^k\|z_{j-1}-z^*\|_2^2\to 0$ implying $\|T_4\|_2\to 0$. 
          \textbf{High Level Comments:}
          1. Please see \textcolor{red}{\textbf{Novelty}} above.
          2. Relative cost maximization, \& Robust classification with logistic loss has been shown to have a SC strongly-concave loss in Wood and Dall’Anese, 2022, and [6] below. Any convex-concave SPP with SC regularizer (enforcing $l_2$ sparsity,min norm etc) is a SC strongly-concave SPP. An extension of this work to convex-concave and constrained cases will truly increase its applicability. 
          3. \textcolor{Purple0}{A5.1}: Please see \textbf{ \textcolor{red}{On A5.1}} above.
          4. Please see reply to Q1 of R7.
          5. We will fix the writing. 
          6. We will include more works on SPP including the paper you mentioned.  
\textbf{Detailed Comments:} 
1. \textcolor{Purple0}{A3.4} (modified) $\exists\mathcal{Z}$, a small neighborhood of $z^*$, and a constant $C>0$ such that for $z\in \mathcal{ Z}$, 
$\|H(z)-Q^*(z-z^*)\|_2^2\leq C\|z-z^*\|_2^2$.
2. It should have been $w_{k+1}$. (4) shows that \textcolor{Purple0}{A3.2} and (3) imply that the second moment of $H(z,w)$ does not grow faster than $C(1+\|z-z^*\|_2^2)$ which we use throughout the proofs.
3,4,5,8,11. We will correct these in the updated version. 
6. $Y_i^j$ is a property of $Q^*$, not SEG. In bilinear problem, $Q^*$ has the Hessian of SC regularizers as diagonal blocks and coupling matrix (and its negative) as off-diagonal blocks. 
7. Lm. 15 is for both linear and non-linear case. We will state it at the start of \textcolor{Purple0}{A.1.2}. 
9. Actually the conclusion follows simply from \textcolor{Purple0}{A3.4} since $z_k\to z^*$ a.s. Taylor's expansion is not needed. Will modify.
10. See \textbf{Correctness} above.
\textbf{\textcolor{blue}{R\#10} }
1. Our motivation behind a CLT is to take a step towards constructing confidence interval for the parameter of interest (e.g. Nash equilibrium) which is not possible from expectation convergence. 2. For the proof-techniques novelty, please see \textcolor{red}{\textbf{Novelty}} above.
\textbf{\textcolor{blue}{R\#11}}\textcolor{Purple0}{A3.1}: $Q^*$ is not Hessian. We are solving a SPP, and not an SC minimization. SC function does not have a saddle-point. \textcolor{Purple0}{A3.4,3.5},$V_k$,(8): We will modify the writing. \textcolor{Purple0}{A3.6}: $w_k$ mart-diff implies that noise is mart-diff. We will remove the redundant line in \textcolor{Purple0}{A3.5}. \textcolor{Purple0}{A3.7}: This leads to the Lindeberg's condition for CLT. Remark 3: True. Will update. \textcolor{Purple0}{A5.1}: This is fairly common in controlled MC. Please see \textbf{\textcolor{red}{On A5.1}} above. 
\footnotesize
[1]\url{https://doi.org/10.1016/S0304-4149(00)00085-5}
[2]\url{https://doi.org/10.1007/978-1-4471-3267-7}
[3]\url{https://doi.org/10.48550/arXiv.2005.01350}
[4]\url{https://doi.org/10.1016/S0304-4149(99)00082-4}
[5]\url{https://doi.org/10.1007/978-3-319-97704-1}
[6]\url{https://doi.org/10.48550/arXiv.1910.08623}
\iffalse
[1] Tweedie, R. L. "Drift conditions and invariant measures for MCs." Stochastic processes and their applications 92, no. 2 (2001): 345-354.
[2] Meyn, Sean P., and Richard L. Tweedie. MCs and stochastic stability. Springer Science \& Business Media, 2012.
[3] Wu, Yue Frank, Weitong Zhang, Pan Xu, and Quanquan Gu. "A finite-time analysis of two time-scale actor-critic methods." Advances in Neural Information Processing Systems 33 (2020): 17617-17628.
[4] Jarner, Søren Fiig, and Ernst Hansen. "Geometric ergodicity of Metropolis algorithms." Stochastic processes and their applications 85, no. 2 (2000): 341-361.
[5]Douc, Randal, Eric Moulines, Pierre Priouret, and Philippe Soulier. MCs. Cham, Switzerland: Springer International Publishing, 2018.
[6]Esfandiari, Yasaman, Aditya Balu, Keivan Ebrahimi, Umesh Vaidya, Nicola Elia, and Soumik Sarkar. "A fast saddle-point dynamical system approach to robust deep learning." Neural Networks 139 (2021): 33-44.
\fi

Correctness. Please look at the equation 2 lines above (36) (one line above (a)) where we have $\|T_4\|_2\leq k^{-1/2}\sum_{j=1}^k\eta_j\|\sum_{i=j}^kY_j^i\|_2\|H(z_{j-1})-Q^*V_{j-1}\|_2$. Expressions $\|T_4\|_2\leq \lesssim k^{-1/2}\sum_{j=1}^k\|H(z_{j-1})-Q^*V_{j-1}\|_2$ or $\|T_4\|_2\lesssim k^{-1/2}\sum_{j=1}^k\|z_{j-1}-z^*\|_2^2$ trivially follow from that line when one uses Lemma 14, and Assumption 3.4 as we have stated just below (36). We had merely skipped the intermediate steps as it seemed trivial but the argument is correct.
The bound in (a) and the line after is correct as well. It simply follows from the fact that j<=k, and consequently, $1/j^0.5>=1/k^0.5$. Note that, since $j \leq k$, $\|T_4\|_2\lesssim k^{-1/2}\sum_{j=1}^k\|z_{j-1}-z^*\|_2^2 \leq \sum_{j=1}^kj^{-1/2}\|z_{j-1}-z^*\|_2^2$. 

1. NOVELTY: The papers you cited study different problem from ours in different settings. Denote: A=https://arxiv.org/abs/2209.08005, B=https://arxiv.org/pdf/1105.4681.pdf.  The main differences are:
a) In both the papers, the transition kernel P of the Markov chain does not depend on the current iterate ($w_t$ in A, $x_t$ in B) whereas we deal with state-dependent Markov noise. 

b) Because of the state independence, neither A nor B run into any stability problem which is not the case for us. We have already pointed out why showing the stability and the associated analysis to establish CLT for SPP is nontrivial.

c) They both assume the data is exponentially mixing Markov chain, i.e., for some distance measure d, $d(P^t,\pi^*)<= a^t$ where $0<a<1$ (Assumption 1 and Lemma A.1 in A, Assumption D in B). B also shows a result for polynomially mixing assumption. These assumptions is easier to deal with, as B themselves explain on top of page 23, since these assumptions imply that the data samples separated by a few time steps become almost independent. We do not assume such mixing conditions for the data sequence. Note that Assumption 5.1.1 implies V-uniform ergodicity only for fixed $\theta$, but the mixing properties of the chain is completely controlled by $\theta$ as the chain evolves.

d) "A" studies stability and generalization properties of SGD and SGDA whereas B studies expected convergence of SGD. None of them establishes CLT for Saddle Point Problem for martingale-difference and State-dependent Markov noise for Stochastic Extra-gradient algorithm. 

We request you to kindly point us to some specific reference where a CLT has been established for Stochastic Extra-gradient algorithm when applied to Saddle Point Problem under martingale-difference and State-dependent Markov noise.

3. The papers we cited have shown the applications with state-dependent Markov noise and verified Assumption 5.1.1 for those applications. Here we present the relative cost maximization in competitive market for electric vehicle charging 
(Wood and Dall’Anese, 2022). 

EXAMPLE: We consider the game where there are two competing service providers A and B for EV charging aiming to maximize their relative profits over n zones.  At each zone $i$ there is an average
baseline price $p_i$. The provider sets the price differential $x_i$ to charge per-minute. 
For provider A,
Demand = $a_i$
Revenue=$a_i(x_i+p_i)$
Zone-based utility cost= $\theta_i(x_i+p_i)$.
Quality of service cost which penalizes large deviation from baseline = $\gamma_{A,i}x_i^2$, $\gamma_{A,i}>0$.
Similarly, for provider B, 
Demand = $b_i$
Revenue=$b_i(y_i+p_i)$
Zone-based utility cost= $\theta_i(y_i+p_i)$.
Quality of service cost which penalizes large deviation from baseline = $\gamma_{B,i}y_i^2$, $\gamma_{B,i}>0$.

The distribution of demand $(a_k,b_k)$ at time $k$ is shown to linearly depend on $(x_{k-1},y_{k-1})$ (Wood and Dall’Anese, 2022) as well as the demand at the previous time step $(a_{k-1},b_{k-1})$ (see [3,4] below). So the demands are modeled to be sampled from, 
$a_{k+1}~D_A+\rho a_{k}+A_1x_k+A_2y_k$, $b_{k+1}~D_B+\rho b_{k}+B_1x_k+B_2y_k$ where elements of $A_1$($A_2$) are negative(positive), $B_1=A_2$, $B_2=A_1$,  $D_A,D_B$ is some prior distribution for which the $2+\epsilon$ moments exist for arbitrarily small $\epsilon>0$, and $0<\rho<1$. As explained in Wood and Dall’Anese, 2022, the objective of the optimization is independent of $p_i$. So we remove $p_i$. To enforce smaller values of $x$ and $y$, we use regularization parameters $lambda$, $\beta$ instead of constraints since we consider the unconstrained version of the problem. So the optimization problem can be written in the following way which is a Strongly-convex strongly-concave saddle point problem. 
\begin{align*}
    \min_{x\in R^n} \max_{y\in R^n} E[||\Gamma_A x||_2^2-||\Gamma_B y||_2^2-x^\top (a+\theta)+y^\top (b+\theta)+\lambda ||x||_2^2-\beta ||y||_2^2],
\end{align*}
where the expectation is w.r.t $a$ and $b$, $\Gamma_A=diag{\gamma_A^i}$, $\Gamma_B=diag{\gamma_B^i}$. In the above expression we omit the subscript $i$ to denote the vector. 

Verification of Assumption 5.1
It is easy to see that the noise $(a_k,b_k)$ is state-dependent Markov noise. Since $2+\epsilon$ moments exist for the noise, $\mathcal{V}(a,b)$ in Assumption 5.1 can be chosen as $||a||+||b||$. Then, $E(V^\alpha)<\infty$ for $\alpha=2+\epsilon$.

A5.1.1 
Since $0<\rho<1$, when $x$ and $y$ are fixed, the chain is geometrically ergodic (proved in Proposition 3 of [5] below) thus satisfying our Assumption 5.1.1. 

A5.1.2 
When $(x,y)$ belongs to a compact set, the gradient is a linear function of noise which can be upper bounded by the order of $\mathcal{V}$ as defined above. Since the gradient of the objective is linear, the gradient is Lipschitz continuous satisfying second part of Assumption 5.1.2. 

A.5.1.3 
Since the transition kernel is linear in $x$ and $y$ the Lipschitz property holds verifying Assumption 5.1.3. 

 


4. We are not completely sure what you mean here. We said that the results are possibly extendable to SGDA which provably converges in the strongly-convex and strongly-concave case. We said that SGDA may not converge (shown in [1] below) for convex-concave problem (NOT strongly-convex strongly-concave). But SEG does converge in convex-concave problem (shown in [1]). Keeping this broader application of SEG in mind, we analyzed SEG to take a step forward towards inference of convex-concave problems in future. 



[1] Mokhtari, Aryan, Asuman Ozdaglar, and Sarath Pattathil. "A unified analysis of extra-gradient and optimistic gradient methods for saddle point problems: Proximal point approach." In International Conference on Artificial Intelligence and Statistics, pp. 1497-1507. PMLR, 2020.
[2] Li, Qiang, and Hoi-To Wai. "State dependent performative prediction with stochastic approximation." In International Conference on Artificial Intelligence and Statistics, pp. 3164-3186. PMLR, 2022.
[3] Yan, Qingyou, Hongyu Lin, Jinmeng Li, Xingbei Ai, Mengshu Shi, Meijuan Zhang, and De Gejirifu. "Many-objective charging optimization for electric vehicles considering demand response and multi-uncertainties based on Markov chain and information gap decision theory." Sustainable Cities and Society 78 (2022): 103652.
[4]Zhang, Li, and Zheng He. "Spatiotemporal Distribution Model of Charging Demand for Electric Vehicle Charging Stations Based on Markov Chain." In Journal of Physics: Conference Series, vol. 1601, no. 2, p. 022045. IOP Publishing, 2020.
[5] Grunwald, Gary K., Rob J. Hyndman, Leanna Tedesco, and Richard L. Tweedie. "Theory \& Methods: Non‐Gaussian Conditional Linear AR (1) Models." Australian \& New Zealand Journal of Statistics 42, no. 4 (2000): 479-495.
